# Supplementary material for: Beam engineering for selective and enhanced coupling to multipolar resonances
Source: arXiv:1509.01281 source file (2015-09-03)
Supplement: Supplementary file 1 [file PRL_beam_engineering_supplement.pdf]

# Supplementary Materials:
# Beam engineering for selective and enhanced coupling to multipolar resonances

Tanya Das, Prasad P. Iyer, and Jon A. Schuller

This supplement provides expressions for the electric and magnetic fields both internal and external to a spherical particle under illumination by any kind of incident beam in section I, which relies on expressing the incident beam as a summation of plane waves. From these expressions, the scattered, extinction, and absorbed power are calculated for the dipole and quadrupole modes in section II, and these expressions are shown to have an explicit dependence on the local field properties at the location of the particle within the beam. Additionally, the issues with discretization of the incident beam in calculating the incident power of the beam is discussed in section III. The results for the scattering spectra obtained using the local field method presented in the main text are compared with published results obtained using the Generalized Lorenz Mie theory in section IV, and the two are shown to have excellent agreement.

## I. INCIDENT, SCATTERED, AND INTERNAL ELECTRIC AND MAGNETIC FIELDS

In this section, expressions are derived for the internal and scattered electric and magnetic fields of a spherical particle under illumination by an arbitrary incident beam. Expressions for the electric and magnetic fields of the arbitrary incident beams are also derived, and are expressed both as a summation plane waves (plane wave spectrum, or PWS), and a subsequent expansion into spherical vector harmonics (SVHs).

### A. Incident electric and magnetic fields

Any arbitrary incident beam can be expressed as a summation of plane waves, as is the convention in the plane wave spectrum technique [1, 2]. The angular spectrum representation [3] of such a beam is given as,

$$\mathbf{E}_{inc}(\mathbf{r}) = \int_0^{2\pi} \int_0^{\alpha} \widehat{E}(\theta, \phi) e^{i\mathbf{k}\cdot\mathbf{r}} \sin\theta d\theta d\phi \tag{1}$$

Here, $\widehat{E}(\theta, \phi)$ is the angular spectrum for the incident beam, $\mathbf{k}\cdot\mathbf{r} = k(\sin\theta\cos\phi x + \sin\theta\sin\phi y + \cos\theta z)$ where $k$ is the wavenumber of the wave in the medium, and $\alpha$ is the collection angle of a

lens for a focused wave. The vector $\mathbf{r}$ describes the position of the nano particle (NP) within the beam. This integral may be consequently converted to a summation as,

$$\mathbf{E}\ (\mathbf{r}) = \lim_{N_\theta, N_\phi \to \infty} \sum_{i=1}^{N_\theta} \sum_{j=1}^{N_\phi} \widehat{E}(\theta_i, \phi_i) e^{i\mathbf{k}\cdot\mathbf{r}} d\theta_i d\phi_i \tag{2}$$

where $d\theta_i = \frac{\alpha}{N_\theta}$ and $d\phi_i = \frac{2\pi}{N_\phi}$. Taking a finite number of plane waves $N_\theta$ and $N_\phi$, the integral in equation (1) is approximated by a discrete summation of plane waves with varying polarization, angle of incidence, and complex amplitude, each given by a pair of rotation angles $\theta_i$ and $\phi_j$. By fixing the location of the NP within the beam $\mathbf{r}$, this discrete summation becomes a summation of plane waves with varying polarization and complex amplitude.

The convention in Mie theory, which fully describes the interaction between a plane wave and a spherical NP, is that the plane wave be x-polarized and incident along the z-axis [4]. Here, we describe the incident beam as a collection of plane waves with arbitrary polarization and angle of incidence. We treat each incident plane wave as if, in a local coordinate system which is specific to each wave, it is x-polarized and incident along the z-axis. Then, using rotation angles, each plane wave in the angular spectrum may be expressed using rotation angles about the y- ($\theta_p$) and z- ($\phi_p$) axes, to translate each wave from being polarized along the x-axis and incident along the z-axis in a local coordinate system, to being arbitrarily polarized in a main coordinate system, as depicted in Fig. 1.

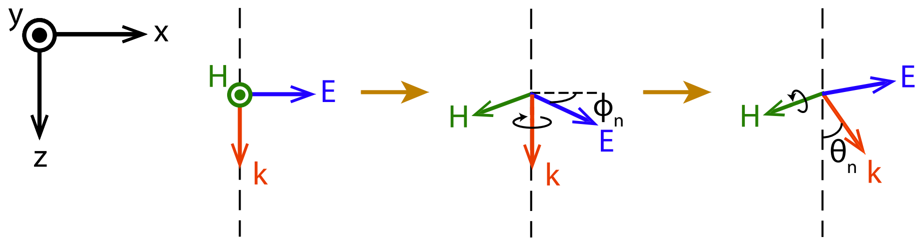


FIG. 1: In order to translate waves from being polarized along the x-axis and incident along the z-axis in a local coordinate system, to being oriented in some arbitrary direction in a main coordinate system, each plane wave in angular spectrum is described by two rotation angles about the y- and z-axes.

Using this convention, the the electric field due to the $p^{th}$ plane wave in the summation is given by equation (3), in which $\mathbf{k_p}$ is the rotated wave vector expressed in the main coordinate system, defined as $k\left(\sin\theta_p\cos\phi_p\hat{e}_x + \sin\theta_p\sin\phi_p\hat{e}_y + \cos\theta_p\hat{e}_z\right)$ and $E_p^{'}$ is the amplitude of the incident plane wave.

$$\mathbf{E}_p = E_p^{'} \left(\cos\theta_p \cos\phi_p \hat{e}_x + \cos\theta_p \sin\phi_p \hat{e}_y - \sin\theta_p \hat{e}_z\right) e^{i\mathbf{k_p}\cdot\mathbf{r}} \tag{3}$$

The particle may be located at any point in the incident beam. By fixing this location $\mathbf{r}$, equation (3) can be rewritten as,

$$\mathbf{E}_p(\mathbf{r}) = E_p \left(\cos\theta_p \cos\phi_p \hat{e}_x + \cos\theta_p \sin\phi_p \hat{e}_y - \sin\theta_p \hat{e}_z\right) \tag{4}$$

where the amplitude of the incident plane wave is written as $E_p$ when the location within the beam is fixed. Thus, for a total number of plane waves $P$, the electric field of the incident beam is given by,

$$\mathbf{E}_{inc}^{PWS} = \sum_{p=1}^{P} E_p \left(\cos\theta_p \cos\phi_p \hat{e}_x + \cos\theta_p \sin\phi_p \hat{e}_y - \sin\theta_p \hat{e}_z\right) \tag{5}$$

Alternatively, the plane waves in (5) could be expanded into SVHs, and the resulting expression for the electric field of the incident beam is given by,

$$\mathbf{E}_{inc}^{SVH} = \sum_{p=1}^{P} \sum_{l=1}^{\infty} E_l E_p \left(R_{li}^{M} \mathbf{M}_{o1l}^{p} - i R_{li}^{N} \mathbf{N}_{e1l}^{p}\right) \tag{6}$$

which is adapted from equation (4.37) in reference [4], and the exact expressions for the SVHS are provided in (19)-(22). Here, $E_l = i^l \frac{2l+1}{l(l+1)}$, where $l$ refers to the mode order, in the context of Mie Theory. $R_{li}^{N}$ describes the radial dependence, and is defined as,

$$R_{li,s}^{N} = \begin{cases} \psi_l^{'}\left(\rho\right)/\rho \text{ for incoming } (i) \text{ fields} \\ \xi_l^{'}\left(\rho\right)/\rho \text{ for scattered } (s) \text{ fields} \end{cases} \quad R_{li,s}^{M} = \begin{cases} \psi_l\left(\rho\right)/\rho \text{ for incoming } (i) \text{ fields} \\ \xi_l\left(\rho\right)/\rho \text{ for scattered } (s) \text{ fields} \end{cases} \tag{7}$$

where $\psi_l$ and $\xi_l$ are the Riccati-Bessel functions, and $\rho = kr$. The $p$ superscripts on $\mathbf{M}_{o1l}$ and $\mathbf{N}_{e1l}$ indicate that these SVHs include rotation information, which are defined explicitly in later sections. We ignore the radial vector component of the $\mathbf{N}$ SVHs for simplicity, since only the $\hat{e}_\theta$ and $\hat{e}_\phi$ components of the SVHs are needed for our derivations.

Similarly, the magnetic field of the incident beam can be expressed as a summation of plane waves and as a subsequent expansion into SVHs, given by,

$$\mathbf{H}_{inc}^{PWS} = \frac{k}{\omega\mu}\sum_{p=1}^{P} E_p\left(-\sin\phi_p \hat{e}_x + \cos\phi_p \hat{e}_y\right) \tag{8}$$

$$\mathbf{H}_{inc}^{SVH} = -\frac{k}{\omega\mu}\sum_{p=1}^{P}\sum_{l=1}^{\infty} E_l E_p\left(R_{li}^M \mathbf{M}_{e1l}^p + iR_{li}^N \mathbf{N}_{o1l}^p\right) \tag{9}$$

### B. Internal and scattered electric and magnetic fields

Using the formulation provided in section I A, the electric and magnetic fields internal to the particle are given by,

$$\mathbf{E}_{int} = \sum_{p=1}^{P}\sum_{l=1}^{\infty} E_l E_p\left(c_l R_{li}^M \mathbf{M}_{o1l}^p - id_l R_{li}^N \mathbf{N}_{e1l}^p\right) \tag{10}$$

$$\mathbf{H}_{int} = -\frac{k_{np}}{\omega\mu_{np}}\sum_{p=1}^{P}\sum_{l=1}^{\infty} E_l E_p\left(d_l R_{li}^M \mathbf{M}_{e1l}^p + ic_l R_{li}^N \mathbf{N}_{o1l}^p\right) \tag{11}$$

where $k_{np}$ refers to the wave number inside the particle and $\mu_{np}$ refers to the magnetic permeability inside the particle.

Similarly, the scattered electric and magnetic fields are given by,

$$\mathbf{E}_{sca} = \sum_{p=1}^{P}\sum_{l=1}^{\infty} E_l E_p\left(ia_l R_{ls}^N \mathbf{N}_{e1l}^p - b_l R_{ls}^M \mathbf{M}_{o1l}^p\right) \tag{12}$$

$$\mathbf{H}_{sca} = \frac{k}{\omega\mu}\sum_{p=1}^{P}\sum_{l=1}^{\infty} E_l E_p\left(ib_l R_{ls}^N \mathbf{N}_{o1l}^p + a_l R_{ls}^M \mathbf{M}_{e1l}^p\right) \tag{13}$$

The coefficients $a_l, b_l, c_l$ and $d_l$ refer to the appropriate Mie coefficients obtained by applying the Maxwell boundary conditions, and are defined in [4]. Using these expressions, the scattered, extinction, and absorbed power may be derived for the dipole and quadrupole modes, given in section II, and are shown to depend on specific field properties for each type of mode.

## II. SCATTERED, EXTINCTION, AND ABSORBED POWER

In this section, expressions are provided for the scattered, extinction, and absorbed power of the electric and magnetic dipole and quadrupole modes. The expressions are derived for the electric modes explicitly, while the derivations for the magnetic modes follow straightforwardly from the information contained within. These expressions demonstrate an explicit dependence upon the properties of the illuminating field, where the illuminating field magnitudes are shown to drive the dipole mode interactions, and the illuminating field gradients are shown to drive the quadrupole mode interactions.

### A. Scattered power: dipole modes

As mentioned previously, the power scattered by the electric dipole mode is derived explicitly, and the expression for the power scattered by the magnetic dipole mode is provided. In order to calculate the power scattered by the electric dipole mode, the scattered electric and magnetic fields for the electric dipole mode are required. These may be obtained from equations (12) and (13), in which the mode order is chosen as $l = 1$, as these correspond to the dipole modes, and the $a_n$ Mie coefficients are chosen, as these correspond to the electric modes. The resulting expressions for the scattered electric and magnetic fields are given by,

$$\mathbf{E}_{sca}^{ED} = \sum_{p=1}^{P} E_{l=1} E_p \left( i a_1 R_{1s}^{N} \mathbf{N}_{e11}^{p} \right) = E_{EDs} \sum_{p=1}^{P} E_p \mathbf{N}_{e11}^{p} \tag{14}$$

$$\mathbf{H}_{sca}^{ED} = \frac{k}{\omega\mu} \sum_{p=1}^{P} E_{l=1} E_p \left( a_1 R_{1s}^{M} \mathbf{M}_{e11}^{p} \right) = H_{EDs} \sum_{p=1}^{P} E_p \mathbf{M}_{e11}^{p} \tag{15}$$

where $E_{EDs} = i a_1 E_{l=1} R_{1s}^{N} = -a_1 \frac{3}{2} \frac{\xi_1'(kr)}{kr}$ and $H_{EDs} = a_1 \frac{k}{\omega\mu} E_{l=1} R_{1s}^{M} = i a_1 \frac{k}{\omega\mu} \frac{3}{2} \frac{\xi_1(kr)}{kr}$. The notation here differs from [4] in that the radial dependence of the SVHs is expressed independently. The scattered power is then calculated from the scattered electric and magnetic fields as,

$$P_{sca} = \frac{1}{2} \text{Re} \int_0^{2\pi} \int_0^{\pi} (E_{s\theta} H_{s\phi}^* - E_{s\phi} H_{s\theta}^*) r^2 \sin\theta d\theta d\phi \tag{16}$$

Using equations (14) and (15) in (16) gives (17),

$$P_{sca}^{ED} = \frac{1}{2}\mathrm{Re}\ E_{EDs}H_{EDs}^{*}\int_{0}^{2\pi}\int_{0}^{\pi}\left[\left(E_1 N_{e11\theta}^{1} + ... + E_P N_{e11\theta}^{P}\right)\left(E_1^{*} M_{e11\phi}^{1*} + ... + E_P^{*} M_{e11\phi}^{P*}\right)\right. \\ \left. - \left(E_1 N_{e11\phi}^{1} + ... + E_P N_{e11\phi}^{P}\right)\left(E_1^{*} M_{e11\theta}^{1*} + ... + E_P^{*} M_{e11\theta}^{P*}\right)\right] r^2 \sin\theta d\theta d\phi \tag{17}$$

Explicitly performing the multiplications in (17) gives,

$$P_{sca}^{ED} = \mathrm{Re}\ W_{EDs}\int_{0}^{2\pi}\int_{0}^{\pi}\Big[|E_1|^2\left(N_{e11\theta}^{1}M_{e11\phi}^{1*} - N_{e11\phi}^{1}M_{e11\theta}^{1*}\right) + ... + |E_P|^2\left(N_{e11\theta}^{P}M_{e11\phi}^{P*} - N_{e11\phi}^{P}M_{e11\theta}^{P*}\right) + \\ E_1E_2^{*}\left(N_{e11\theta}^{1}M_{e11\phi}^{2*} - N_{e11\phi}^{1}M_{e11\theta}^{2*}\right) + ... + E_{P-1}E_P^{*}\left(N_{e11\theta}^{P-1}M_{e11\phi}^{P*} - N_{e11\phi}^{P-1}M_{e11\theta}^{P*}\right) + \\ E_2E_1^{*}\left(N_{e11\theta}^{2}M_{e11\phi}^{1*} - N_{e11\phi}^{2}M_{e11\theta}^{1*}\right) + ... + E_PE_{P-1}^{*}\left(N_{e11\theta}^{P}M_{e11\phi}^{P-1*} - N_{e11\phi}^{P}M_{e11\theta}^{P-1*}\right)\Big]\sin\theta d\theta d\phi \tag{18}$$

where $W_{EDs} = \frac{1}{2}E_{EDs}H_{EDs}^{*}r^2$.

This integral is composed of two types, each of which can be solved explicitly. In order to do so, we introduce the exact expressions for the SVHs which are given by,

$$\mathbf{N}_{e11}^{p} = \left(\cos\theta_p\cos\left(\phi - \phi_p\right)\cos\theta + \sin\theta_p\sin\theta\right)\hat{e}_\theta - \cos\theta_p\sin\left(\phi - \phi_p\right)\hat{e}_\phi \tag{19}$$

$$\mathbf{N}_{o11}^{p} = \sin\left(\phi - \phi_p\right)\cos\theta\hat{e}_\theta + \cos\left(\phi - \phi_p\right)\hat{e}_\phi \tag{20}$$

$$\mathbf{M}_{e11}^{p} = -\cos\theta_p\sin\left(\phi - \phi_p\right)\hat{e}_\theta - \left(\cos\theta_p\cos\left(\phi - \phi_p\right)\cos\theta + \sin\theta_p\sin\theta\right)\hat{e}_\phi \tag{21}$$

$$\mathbf{M}_{o11}^{p} = \cos\left(\phi - \phi_p\right)\hat{e}_\theta - \sin\left(\phi - \phi_p\right)\cos\theta\hat{e}_\phi \tag{22}$$

As such, the first type of integral in (18) is given by equation (23), and can be solved to give,

$$|E_p|^2\int_{0}^{2\pi}\int_{0}^{\pi}\left(N_{e11\theta}^{p}M_{e11\phi}^{p*} - N_{e11\phi}^{p}M_{e11\theta}^{p*}\right)\sin\theta d\theta d\phi = -\frac{8\pi}{3}|E_p|^2 \tag{23}$$

Due to the spherical symmetry of this scattering problem, equation (23) is true for any value of $p$, i.e., for every plane wave in the summation. The second type of integral is given by,

$$\int_{0}^{2\pi}\int_{0}^{\pi}\left[E_pE_q^{*}\left(N_{e11\theta}^{q}M_{e11\phi}^{p*} - N_{e11\phi}^{p}M_{e11\theta}^{q*}\right) + E_qE_p^{*}\left(N_{e11\theta}^{q}M_{e11\phi}^{p*} - N_{e11\phi}^{q}M_{e11\theta}^{p*}\right)\right]\sin\theta d\theta d\phi \tag{24}$$

Using symmetry arguments, it can be shown that $N^q_{e11\theta}M^{p*}_{e11\phi} - N^p_{e11\phi}M^{q*}_{e11\theta} = N^q_{e11\theta}M^{p*}_{e11\phi} - N^q_{e11\phi}M^{p*}_{e11\theta}$. This reduces equation (24) to equation (25), which can also be solved to give,

$$\begin{aligned}&\left(E_pE_q^* + E_qE_p^*\right)\int_0^{2\pi}\int_0^{\pi}\left(N^q_{e11\theta}M^{p*}_{e11\phi} - N^p_{e11\phi}M^{q*}_{e11\theta}\right)\sin\theta d\theta d\phi\\ &= -\frac{8\pi}{3}\left(E_pE_q^* + E_qE_p^*\right)\left(\cos\theta_p\cos\theta_q\cos\left(\phi_p-\phi_q\right)+\sin\theta_p\sin\theta_q\right)\end{aligned} \tag{25}$$

Thus the expression for the power scattered by the electric dipole mode (18) reduces to,

$$P^{ED}_{sca} = -\text{Re }W_{EDs}\frac{8\pi}{3}\sum_{p=1}^{P}\sum_{q\neq p}|E_p|^2 + \left(E_pE_q^* + E_qE_p^*\right)\left(\cos\theta_p\cos\theta_q\cos\left(\phi_p-\phi_q\right)+\sin\theta_p\sin\theta_q\right) \tag{26}$$

We previously defined $W_{EDs} = \frac{1}{2}E_{EDs}H^*_{EDs}r^2 = -i\frac{9}{8}|a_1|^2\frac{1}{k\omega\mu}\xi_1\xi_1'^*$. Since we are dealing with far-field expressions, we take the limit for large $kr$: $\lim_{kr\to\infty}\xi_1\xi_1'^* = -i$. Inserting this into equation (26) gives our final expression for the power scattered by the electric dipole mode to be,

$$P^{ED}_{sca} = \frac{3\pi}{k\omega\mu}|a_1|^2\sum_{p=1}^{P}\sum_{q\neq p}|E_p|^2 + \left(E_pE_q^* + E_qE_p^*\right)\left(\cos\theta_p\cos\theta_q\cos\left(\phi_p-\phi_q\right)+\sin\theta_p\sin\theta_q\right) \tag{27}$$

To simply this expression further we turn to our original expression for the incident electric field. Using equation (5), we can calculate the magnitude of the incident electric field as follows:

$$\begin{aligned}|\mathbf{E}_{inc}|^2 &= |E_{inc,x}|^2 + |E_{inc,y}|^2 + |E_{inc,z}|^2\\ |E_{inc,x}|^2 &= \sum_{p=1}^{P}\sum_{q\neq p}|E_p|^2\cos\theta_p{}^2\cos\phi_p{}^2 + \left(E_pE_q^* + E_p^*E_q\right)\left(\cos\theta_p\cos\theta_q\cos\phi_p\cos\phi_q\right)\\ |E_{inc,y}|^2 &= \sum_{p=1}^{P}\sum_{q\neq p}|E_p|^2\cos\theta_p{}^2\sin\phi_p{}^2 + \left(E_pE_q^* + E_p^*E_q\right)\left(\cos\theta_p\cos\theta_q\sin\phi_p\sin\phi_q\right)\\ |E_{inc,z}|^2 &= \sum_{p=1}^{P}\sum_{q\neq p}|E_p|^2\sin\theta_p{}^2 + \left(E_pE_q^* + E_p^*E_q\right)\left(\sin\theta_p\sin\theta_q\right)\end{aligned}$$

$$\implies |\mathbf{E}_{inc}|^2 = \sum_{p=1}^{P}\sum_{q\neq p}|E_p|^2 + \left(E_pE_q^* + E_qE_p^*\right)\left(\cos\theta_p\cos\theta_q\cos\left(\phi_p-\phi_q\right)+\sin\theta_p\sin\theta_q\right) \tag{28}$$

We see that (27) is simplified by (28) and our final expression for the power scattered by the electric dipole mode is directly given by the magnitude of the incident electric field as,

$$P_{sca}^{ED} = \frac{3\pi}{k\omega\mu}|a_1|^2|\mathbf{E}_{inc}|^2 \tag{29}$$

The power scattered by the magnetic dipole mode may be derived similarly, and is given by,

$$P_{sca}^{MD} = \frac{3\pi}{k\omega\mu}|b_1|^2 Z^2|\mathbf{H}_{inc}|^2 \tag{30}$$

where $Z$ is the impedance of the medium

### B. Extinction and absorbed power: dipole modes

The extinction power for the electric dipole mode is derived explicitly and the expression for the extinction power of the magnetic dipole mode is provided. In order to calculate the extinction power of the electric dipole mode, the electric and magnetic field components of the incident beam that drive the electric dipole interaction are required, as well as the scattered electric and magnetic fields for the electric dipole mode. The latter are given in (14) and (15). The former may be obtained from (6) and (9), in which the mode order is chosen as $l = 1$ and the even SVHs are chosen ($\mathbf{N}$ for the electric field and $\mathbf{M}$ for the magnetic field), as these correspond to the electric dipole mode. The resulting expressions for the incident electric and magnetic fields driving the electric dipole interaction are given by,

$$\mathbf{E}_{inc}^{ED} = \sum_{p=1}^{P} E_{l=1}E_p\left(-iR_{1i}^N\mathbf{N}_{e11}^p\right) = E_{EDi}\sum_{p=1}^{P} E_p\mathbf{N}_{e11}^p \tag{31}$$

$$\mathbf{H}_{inc}^{ED} = -\frac{k}{\omega\mu}\sum_{p=1}^{P} E_{l=1}E_p\left(R_{1i}^M\mathbf{M}_{e11}^p\right) = H_{EDi}\sum_{p=1}^{P} E_p\mathbf{M}_{e11}^p \tag{32}$$

where $E_{EDi} = -iE_{l=1}R_{1i}^N = \frac{3}{2}\frac{\psi_1'(kr)}{kr}$ and $H_{EDi} = -\frac{k}{\omega\mu}E_{l=1}R_{1i}^M = -i\frac{k}{\omega\mu}\frac{3}{2}\frac{\psi_1(kr)}{kr}$.

The extinction power is given by,

$$P_{ext} = \frac{1}{2}\mathrm{Re}\int_0^{2\pi}\int_0^{\pi}(E_{i\phi}H_{s\theta}^* - E_{i\theta}H_{s\phi}^* - E_{s\theta}H_{i\phi}^* + E_{s\phi}H_{i\theta}^*)r^2\sin\theta d\theta d\phi \tag{33}$$

Using equations (14)-(15) and (31)-(32) in (33) gives,

$$P_{ext}^{ED} = \frac{1}{2}\text{Re }\left(E_{EDi}H_{EDs}^* + E_{EDs}H_{EDi}^*\right)\int_0^{2\pi}\int_0^{\pi}\left[\left(E_1 N_{e11\theta}^1 + ... + E_P N_{e11\theta}^P\right)\left(E_1^* M_{e11\phi}^{1*} + ... + E_P^* M_{e11\phi}^{P*}\right)\right.$$
$$\left. - \left(E_1 N_{e11\phi}^1 + ... + E_P N_{e11\phi}^P\right)\left(E_1^* M_{e11\theta}^{1*} + ... + E_P^* M_{e11\theta}^{P*}\right)\right] r^2 \sin\theta d\theta d\phi \tag{34}$$

The integral in equation (34) is the same as that in equation (17), which has already been solved. Thus we can rewrite the extinction power of the electric dipole mode as,

$$P_{ext}^{ED} = -\text{Re } W_{EDe}\frac{8\pi}{3}\sum_{p=1}^{P}\sum_{q\neq p}|E_p|^2 + \left(E_p E_q^* + E_q E_p^*\right)\left(\cos\theta_p\cos\theta_q\cos\left(\phi_p - \phi_q\right) + \sin\theta_p\sin\theta_q\right) \tag{35}$$

where the prefactor can be simplified as follows,

$$\begin{aligned}
\text{Re }\left(W_{EDe}\right) &= \text{Re }\frac{1}{2}\left(E_{EDi}H_{EDs}^* + E_{EDs}H_{EDi}^*\right)r^2 \\
&= \text{Re }\frac{1}{k\omega\mu}\frac{9}{8}\left(ia_1^*\psi_1^{'}\xi_1^* + ia_1\xi_1^{'}\psi_1^*\right) \\
&= \text{Re }\frac{1}{k\omega\mu}\frac{9}{8}\left(ia_1^*\psi_1^{'}\left(\psi_1^* + i\chi_1^*\right) + ia_1(\psi_1^{'} - i\chi_1^{'})\psi_1^*\right) \\
&= \frac{1}{k\omega\mu}\frac{9}{8}\text{Re}\left(i(a_1^* + a_1)\psi_1^{'}\psi_1^* - a_1^*\psi_1^{'}\chi_1^* + a_1\chi_1^{'}\psi_1^*\right) \\
&= \frac{1}{k\omega\mu}\frac{9}{8}\left(\text{Re}(a_1)\text{Im}(\psi_1^{'}\psi_1^*) - \text{Re}(a_1)\text{Re}\left(\psi_1^{'}\chi_1^* - \chi_1^{'}\psi_1^*\right)\right) \\
&= -\frac{1}{k\omega\mu}\frac{9}{8}\text{Re}(a_1)
\end{aligned} \tag{36}$$

Here, the last step follows since $\psi_n$ is always real for real argument, and $\psi_n^{'}\chi_n^* - \chi_n^{'}\psi_n^* = 1$. Inserting this back into (35), and using the definition for the magnitude of the incident electric field in (28), the expression for the extinction power of the electric dipole mode simplifies to,

$$P_{ext}^{ED} = \frac{3\pi}{k\omega\mu}\text{Re}\left(a_1\right)|\mathbf{E}_{inc}|^2 \tag{37}$$

and once again the dipole mode is shown to be driven by the incident electric field magnitude. The extinction power of the magnetic dipole mode may be derived similarly, and is given by,

$$P_{ext}^{ED} = \frac{3\pi}{k\omega\mu}\text{Re}\left(b_1\right)Z^2|\mathbf{H}_{inc}|^2 \tag{38}$$

where $Z$ is the impedance of the medium.

Correspondingly, the absorbed power for the dipole modes is obtained from the scattered and extinction power equations, and is given by,

$$W_{abs} = W_{ext} - W_{sca} \tag{39}$$

where $P_{sca}$ and $P_{ext}$ are given in equations (29), (37) and (30), (38) for the electric and magnetic dipoles, respectively.

### C. Scattered power: quadrupole modes

In this section, the power scattered by the electric quadrupole mode is derived explicitly, and the expression for the power scattered by the magnetic quadrupole mode is provided. Similar to the derivation for the power scattered by the electric dipole mode, we begin by obtaining expressions for the scattered electric and magnetic fields for the electric quadrupole mode. These may be obtained from equations (12) and (13), in which the mode order is chosen as $l = 2$, as these correspond to the quadrupole modes, and the $a_n$ coefficient are chosen, as these correspond to the electric modes. The resulting expressions for the scattered electric and magnetic fields for the electric quadrupole modes are given by,

$$\mathbf{E}_{sca}^{EQ} = \sum_{p=1}^{P} E_{l=2} E_p \left( i a_2 R_{2s}^N \mathbf{N}_{e12}^p \right) = E_{EQs} \sum_{p=1}^{P} E_p \mathbf{N}_{e12}^p \tag{40}$$

$$\mathbf{H}_{sca}^{EQ} = \frac{k}{\omega\mu} \sum_{p=1}^{P} E_{l=2} E_p \left( a_2 R_{2s}^M \mathbf{M}_{e12}^p \right) = H_{EQs} \sum_{p=1}^{P} E_p \mathbf{M}_{e12}^p \tag{41}$$

where $E_{EQs} = i a_2 E_{l=2} R_{2s}^N = -i a_2 \frac{5}{6} \frac{\xi_2'(kr)}{kr}$ and $H_{EQs} = a_2 \frac{k}{\omega\mu} E_{l=2} R_{2s}^M = -a_2 \frac{k}{\omega\mu} \frac{5}{6} \frac{\xi_2(kr)}{kr}$. The scattered power is then calculated from (16) to give an expression very similar to equation (17), in which we simply replace $N_{e11}, M_{e11}$ with $N_{e12}, M_{e12}$. The explicit expressions for $\mathbf{N}_{e12}^p$ and $\mathbf{M}_{e12}^q$ are given by,

$$\begin{aligned} \mathbf{N}_{e12}^p = &\left( 3\cos 2\theta_p \cos 2\theta \cos(\phi - \phi_p) + \frac{3}{4}\left(3 + \cos\left[2(\phi - \phi_p)\right]\right) \sin 2\theta_p \sin 2\theta \right) \hat{e}_\theta \\ &- 3\left(\cos 2\theta_p \cos\theta + \cos(\phi - \phi_p) \sin 2\theta_p \sin\theta\right) \sin(\phi - \phi_p) \hat{e}_\phi \end{aligned} \tag{42}$$

$$\mathbf{M}^p_{e12} = -3\left(\cos 2\theta_p \cos\theta + \cos(\phi-\phi_p)\sin 2\theta_p \sin\theta\right)\sin(\phi-\phi_p)\hat{e}_\theta \\ -\left(3\cos 2\theta_p\cos 2\theta\cos(\phi-\phi_p)+\frac{3}{4}\left(3+\cos\left[2(\phi-\phi_p)\right]\right)\sin 2\theta_p \sin 2\theta\right)\hat{e}_\phi \tag{43}$$

As was the case in the derivation for the power scattered by the dipole modes, we again have two types of integrals to solve, and the integrals as well as their exact solutions are given below as,

$$|E_p|^2\int_0^{2\pi}\int_0^{\pi}\left(N^p_{e12\theta}M^{p*}_{e12\phi}-N^p_{e12\phi}M^{p*}_{e12\theta}\right)\sin\theta d\theta d\phi = -\frac{72\pi}{5}|E_p|^2 \tag{44}$$

$$\left(E_pE_q^*+E_qE_p^*\right)\int_0^{2\pi}\int_0^{\pi}\left(N^q_{e12\theta}M^{p*}_{e12\phi}-N^p_{e12\phi}M^{q*}_{e12\theta}\right)\sin\theta d\theta d\phi \\ = -\frac{18\pi}{5}\left(E_pE_q^*+E_qE_p^*\right)\left(4\cos 2\theta_p\cos 2\theta_q\cos(\phi_p-\phi_q)+\sin 2\theta_p\sin 2\theta_q\left(3+\cos 2\left(\phi_p-\phi_q\right)\right)\right) \tag{45}$$

Thus the expression for the power scattered by the electric quadrupole mode is given by,

$$P^{EQ}_{sca} = -\text{Re}\ W_{EQs}\frac{18\pi}{5}\sum_{p=1}^{P}\sum_{q\neq p}4|E_p|^2+\left(E_pE_q^*+E_qE_p^*\right)\left(4\cos 2\theta_p\cos 2\theta_q\cos(\phi_p-\phi_q)\right. \\ \left.+\sin 2\theta_p\sin 2\theta_q\left(3+\cos 2\left(\phi_p-\phi_q\right)\right)\right) \tag{46}$$

where we define the prefactor as $W_{EQs} = \frac{1}{2}E_{EQs}H^*_{EQs}r^2 = i\frac{25}{72}|a_2|^2\frac{1}{k\omega\mu}\xi_2\xi_2^{'*}$. Since we are dealing with far-field expressions, we take the limit for large $kr$: $\lim_{kr\to\infty}\xi_2\xi_2^{'*} = -i$. Inserting this into equation (46) gives our final expression for the power scattered by the electric quadrupole mode to be,

$$P^{EQ}_{sca} = -\frac{5\pi}{4}\frac{1}{k\omega\mu}|a_2|^2\sum_{p=1}^{P}\sum_{q\neq p}4|E_p|^2+\left(E_pE_q^*+E_qE_p^*\right)\left(4\cos 2\theta_p\cos 2\theta_q\cos(\phi_p-\phi_q)\right. \\ \left.+\sin 2\theta_p\sin 2\theta_q\left(3+\cos 2\left(\phi_p-\phi_q\right)\right)\right) \tag{47}$$

To simply this expression, we calculate the gradient of the incident electric field (reprinted here) along the different Cartesian directions at a fixed point in space.

$$\mathbf{E}_p = E_p^{'}\left(\cos\theta_p\cos\phi_p\hat{e}_x+\cos\theta_p\sin\phi_p\hat{e}_y-\sin\theta_p\hat{e}_z\right)e^{ik(\sin\theta_p\cos\phi_p x+\sin\theta_p\sin\phi_p y+\cos\theta_p z)} \tag{48}$$

The gradient components for each plane wave $p$ in the plane wave summation are given as,

$$\begin{aligned}
\frac{\partial E_x}{\partial x} &= ikE_p \cos\theta_p \sin\theta_p \cos^2\phi_p & \frac{\partial E_x}{\partial y} &= ikE_p \cos\theta_p \sin\theta_p \cos\phi_p \sin\phi_p & \frac{\partial E_x}{\partial z} &= ikE_p \cos^2\theta_p \cos\phi_p \\
\frac{\partial E_y}{\partial x} &= ikE_p \cos\theta_p \sin\theta_p \cos\phi_p \sin\phi_p & \frac{\partial E_y}{\partial y} &= ikE_p \cos\theta_p \sin\theta_p \sin^2\phi_p & \frac{\partial E_y}{\partial z} &= ikE_p \cos^2\theta_p \sin\phi_p \\
\frac{\partial E_z}{\partial x} &= -ikE_p \sin^2\theta_p \cos\phi_p & \frac{\partial E_z}{\partial y} &= -ikE_p \sin^2\theta_p \sin\phi_p & \frac{\partial E_z}{\partial z} &= -ikE_p \sin\theta_p \cos\theta_p
\end{aligned} \tag{49}$$

We define $Q_{ij}$ as the summation of these field gradients, where $i, j$ iterate over the Cartesian components $x, y, z$ and the expression is given by,

$$Q_{ij} = \frac{1}{2}\left(\frac{\partial E_i}{\partial j} + \frac{\partial E_j}{\partial i}\right) \tag{50}$$

Using this expression, each of the $Q_{ij}$ terms are given as,

$$\begin{aligned}
Q_{xx} &= ikE_p \cos\theta_p \sin\theta_p \cos^2\phi_p & Q_{xy} = Q_{yx} &= ikE_p \cos\theta_p \sin\theta_p \cos\phi_p \sin\phi_p \\
Q_{xz} = Q_{zx} &= \frac{ik}{2}E_p \cos 2\theta_p \cos\phi_p & Q_{yy} &= ikE_p \cos\theta_p \sin\theta_p \sin^2\phi_p \\
Q_{yz} = Q_{zy} &= \frac{ik}{2}E_p \cos 2\theta_p \sin\phi_p & Q_{zz} &= -ikE_p \sin\theta_p \cos\theta_p
\end{aligned} \tag{51}$$

Finally, computing summation of the absolute value of $Q_{ij}$ gives,

$$\begin{aligned}
\sum_{i,j} |Q_{i,j}|^2 &= |Q_x x|^2 + ... + |Q_z z|^2 \\
&= -\frac{k^2}{8}\sum_{p=1}^{P}\sum_{q\neq p} 4|E_p|^2 + \left(E_p E_q^* + E_q E_p^*\right)\left(4\cos 2\theta_p \cos 2\theta_q \cos\left(\phi_p - \phi_q\right)\right. \\
&\quad \left. + \sin 2\theta_p \sin 2\theta_q \left(3 + \cos 2\left(\phi_p - \phi_q\right)\right)\right)
\end{aligned} \tag{52}$$

This reduces our expression for the power scattered by the electric quadrupole mode (47) to,

$$P_{sca}^{EQ} = \frac{10\pi}{k^3\omega\mu}|a_2|^2 \sum_{i,j} |Q_{i,j}|^2 \tag{53}$$

and the power scattered by the electric quadrupole mode is directly given by the summation of the incident electric field gradients. The power scattered by the magnetic quadrupole mode may be derived similarly, and is given by,

$$P_{sca}^{MQ} = \frac{10\pi}{k^3\omega\mu}|b_2|^2 Z^2 \sum_{i,j}|G_{i,j}|^2 \tag{54}$$

where $G_{ij}$ is defined analogously to (50), where the electric fields are replaced with magnetic fields.

### D. Extinction and absorbed power: quadrupole modes

The extinction power for the electric quadrupole mode is derived explicitly and the expression for the extinction power of the magnetic quadrupole mode is provided. The procedure is similar to that outlined in section II B, so the extinction power for the electric quadrupole mode is written directly as,

$$\begin{aligned} P_{ext}^{EQ} &= -\text{Re}\ W_{EQe}\frac{18\pi}{5}\sum_{p=1}^{P}\sum_{q\neq p}4|E_p|^2 + \left(E_pE_q^* + E_qE_p^*\right)\left(4\cos 2\theta_p\cos 2\theta_q\cos\left(\phi_p-\phi_q\right)\right. \\ &\left.+\sin 2\theta_p\sin 2\theta_q\left(3+\cos 2\left(\phi_p-\phi_q\right)\right)\right) \end{aligned} \tag{55}$$

in which $W_{EQe} = \frac{1}{2}\left(E_{EQi}H_{EQs}^* + E_{EQs}H_{EQi}^*\right)r^2$, and $E_{EQi}, H_{EQi}$ are given as,

$$\mathbf{E}_{inc}^{EQ} = \sum_{p=1}^{P}E_{l=2}E_p\left(-iR_{2i}^N\mathbf{N}_{e12}^p\right) = E_{EQi}\sum_{p=1}^{P}E_p\mathbf{N}_{e12}^p \tag{56}$$

$$\mathbf{H}_{inc}^{EQ} = -\frac{k}{\omega\mu}\sum_{p=1}^{P}E_{l=2}E_p\left(R_{2i}^M\mathbf{M}_{e12}^p\right) = H_{EQi}\sum_{p=1}^{P}E_p\mathbf{M}_{e12}^p \tag{57}$$

Similarly to before, the prefactor can be simplified as follows,

$$\begin{aligned} \text{Re}\ \left(W_{EQe}\right) &= \text{Re}\ \frac{1}{2}\left(E_{EQi}H_{EQs}^* + E_{EQs}H_{EQi}^*\right)r^2 \\ &= \text{Re}\ \frac{1}{k\omega\mu}\frac{25}{72}\left(ia_2^*\psi_2'\xi_2^* + ia_2\xi_2'\psi_2^*\right) \\ &= \text{Re}\ \frac{1}{k\omega\mu}\frac{25}{72}\left(ia_2^*\psi_2'\left(\psi_2^* + i\chi_2^*\right) + ia_2(\psi_2' - i\chi_2')\psi_2^*\right) \\ &= \frac{1}{k\omega\mu}\frac{25}{72}\text{Re}\left(i(a_2^* + a_2)\psi_2'\psi_2^* - a_2^*\psi_2'\chi_2^* + a_2\chi_2'\psi_2^*\right) \\ &= \frac{1}{k\omega\mu}\frac{25}{72}\left(\text{Re}(a_2)\text{Im}(\psi_2'\psi_2^*) - \text{Re}(a_2)\text{Re}\left(\psi_2'\chi_2^* - \chi_2'\psi_2^*\right)\right) \\ &= -\frac{1}{k\omega\mu}\frac{25}{72}\text{Re}(a_2) \end{aligned} \tag{58}$$

Inserting this back into (55), and using the definition of $Q_{ij}$ in (52), the expression for the extinction power of the electric quadrupole mode simplifies to,

$$P_{ext}^{EQ} = \frac{10\pi}{k^3\omega\mu}\mathrm{Re}\left(a_2\right)\sum_{i,j}|Q_{i,j}|^2 \tag{59}$$

The extinction power of the magnetic quadrupole mode may be derived similarly, and is given by equation as,

$$P_{ext}^{MQ} = \frac{10\pi}{k^3\omega\mu}\mathrm{Re}\left(b_2\right)Z^2\sum_{i,j}|G_{i,j}|^2 \tag{60}$$

And again, the the absorbed power for the dipole modes is obtained from the scattered and extinction power equations, as given in equation (39).

## III. DISCRETIZATION OF INCIDENT BEAM

As was discussed in the main text, the focused incident beams are expressed as a discrete summation of plane waves. All the focused beams in the main text are described as summation of 10,000 total plane waves. The incident power of the illumination beam is calculated by integrating the z-component of the Poynting vector over a ciruclar area, with a specified radius of integration. Even when the radius of integration is quite large (up to 0.1 cm), the incident power does not converge, as is shown in Fig 2. Thus the fraction of scattered to incident power sometimes exceeds 1, since the incident power does not converge even when a large number of plane waves (10,000) are included in the summation that describes the incident beam.

## IV. COMPARISON WITH GLMT

To validate the expressions for the scattered power provided in this text, the ratio of the scattered to incident power is calculated for a gold particle in water under illumination by a focused linearly polarized wave, and compared with published results from [5]. The results obtained using the local field method are given in the shapes (triangle, square, diamond, circle), while the original data, obtained using the Generalized Lorenz Mie theory, is plotted in solid lines, as shown in Fig. 3. The two methods are shown to give excellent agreement.

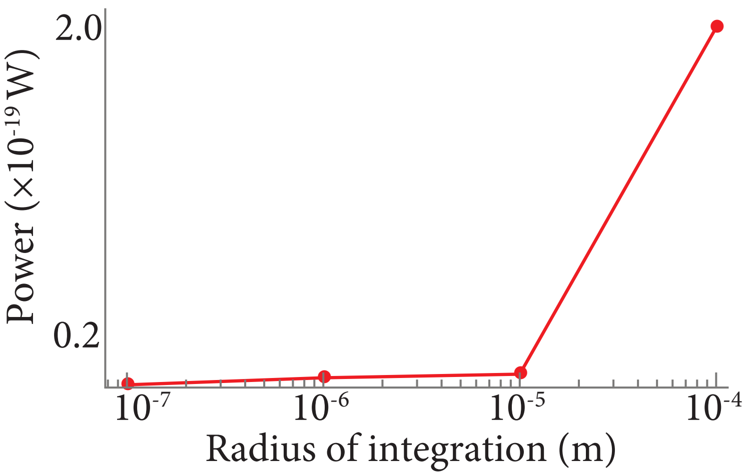


FIG. 2: Power as a function of radius of integration for focused LP beam. Due to the discretization of the incident beam, the power does not converge, even when integrated over a large area.

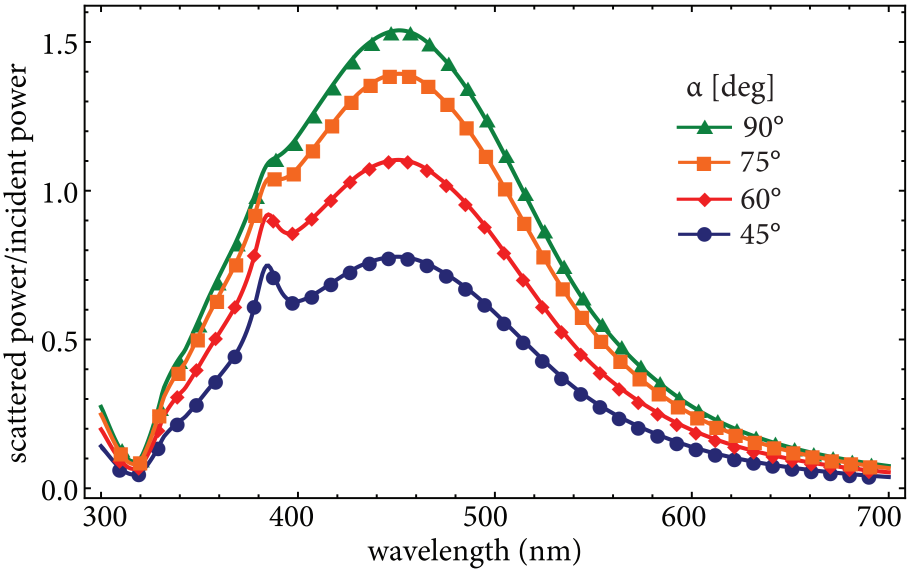


FIG. 3: Fraction of scattered power to incident power of gold spherical NP in water with radius 100nm under focused linearly polarized illumination, as a function of wavelength. Local field results (shapes) are superimposed on GLMT results (solid lines) from [5] at four different focus angles, and the two show excellent agreement.

## V. REFERENCES

[1] J. A. Lock, "Partial-wave expansions of angular spectra of plane waves," *JOSA A*, vol. 23, no. 11, pp. 2803–2809, 2006.

[2] S. Colak, C. Yeh, and L. W. Casperson, "Scattering of focused beams by tenuous particles," *Applied optics*, vol. 18, no. 3, pp. 294–302, 1979.

[3] J. W. Goodman *et al.*, *Introduction to Fourier optics*, vol. 2. McGraw-hill New York, 1968.

[4] C. F. Bohren and D. R. Huffman, *Absorption and scattering of light by small particles.* John Wiley & Sons, 2008.

[5] N. Mojarad, G. Zumofen, V. Sandoghdar, and M. Agio, "Metal nanoparticles in strongly confined beams: transmission, reflection and absorption," *Journal of the European Optical Society-Rapid publications*, vol. 4, 2009.
